# Supplementary material for: X-Class: Text Classification with Extremely Weak Supervision
Source: arXiv:2010.12794 source file (2022-02-07)
Supplement: Supplementary file 1 [file appendix.tex]

% \subsection{Long sentence in BERT}
% We first embed all documents through BERT and get embeddings $E_{ij}$ for each token $t_{ij}$ in a document $D_{i}, i \in \{1, ..., n\}, j \in \{1, ..., L_{i}\}$, where $L_{i}$ is the length of the documents in number of word-pieces. To deal with documents longer than 512 word-pieces, we apply a sliding window of stride 256\footnote{Because of SOS and EOS tokens, in BERT, the actual maximal number of word-pieces is 510, and the sliding window size is 255.}.
